# Supplementary material for: Regularity Learning via Explicit Distribution Modeling for Skeletal Video Anomaly Detection
Source: arXiv:2112.03649 source file (2021-12-08)
Supplement: Supplementary file 1 [file 7_supplementary.tex]

\appendix
In supplementary material, aiming to enhance the confidence of the results in the experiment section and straightforwardly exhibit the model effectiveness, we provide more experimental details of our Motion Prior Regularity Learner (MoPRL) in both quantitative and qualitative aspects. We first explore the model sensitivity through experiments w.r.t. a variety of hyperparameters, including batch size, learning rate, pose embedding dimension, trajectory length, and stride. Further, we provide detailed quantitative visualization to display both success and failure cases of MoPRL. In the end, more analyses based on visualizations are provided for future work.

%%%%%%%%% BODY TEXT - ENTER YOUR RESPONSE BELOW
\section{Hyperparameters Experiments.}

In this section, we investigate the influence brought by different settings of the following hyperparameters: batch size, learning rate, and embedding vector dimension, as well as sliding window length and stride. 
\subsection{Batch Size and Learning Rate.}
According to \cite{devlin2018bert,dosovitskiy2020vit,liu2021Swin}, the common range of learning rate for transformer model training is usually from $1\times10^{-4}$ to $1\times10^{-5}$. Thus, we trained MoPRL under different learning rates in this range to test its sensitivity. From Table~\ref{bs_lr} we notice that MoPRL performs rather steadily w.r.t. batch size when larger learning rate (e.g. $1\times10^{-4}$ or $5\times10^{-5}$) is applied. And it tends to be more prone to batch size when trained with a lower learning rate.

\begin{table}[h]
\centering
\caption{AUC result of MoPRL trained with different batch size and learning rate. Experiment on ShanghaiTech.}
\begin{tabular}{cccc}
\toprule[1pt]
\textbf{\begin{tabular}[c]{@{}c@{}}Learning Rate/\\ Batch Size\end{tabular}} & \textbf{1e-4} & \textbf{5e-5} & \textbf{1e-5} \\ \hline
\textbf{128}                                                                    & 80.99         & 81.22         & 80.39         \\ \hline
\textbf{256}                                                                    & 81.05         & \textbf{81.26}         & 79.42         \\ \hline
\textbf{512}                                                                    & 81.14         & 80.46         & 78.51         \\ \bottomrule[1pt]
\end{tabular}
\label{bs_lr}
\end{table}

\subsection{Sliding Window.}
We utilize the sliding window approach to sample sequences of pose trajectories. As shown in Table \ref{str_trj}, surprisingly, longer sequences do not bring better performance but cause a rapid drop in AUC; on the contrary, when choosing smaller length, the final accuracy keep at a relatively high level and is insensitive to the selected stride. We assume the reason here is that the naive transformer architecture (though process temporal and spatial dimension separately) is not capable of capturing dependencies between distant time steps w.r.t. pose embedding. 

\subsection{Embedding Vector Dimension.}
The pose embedding is an essential component of MoPRL, which encodes the core information of the input data and plays as a bottleneck for the following spatial-temporal transformer. According to Table \ref{emb}, we find that too small an embedding dimension impedes the performance, which indicates that a larger embedding dimension is necessary to encode pose coordinates completely.

\begin{table}[h]
\centering
\caption{AUC result of MoPRL trained with different sliding window setting, including stride and trajectory length. Experiment on ShanghaiTech.}
\begin{tabular}{cccc}
\toprule[1pt]
\textbf{\begin{tabular}[c]{@{}c@{}}Stride/\\Trajectory Length\end{tabular}} & \textbf{1} & \textbf{2} & \textbf{4} \\ \hline
\textbf{4}                                                                      & 79.12      & 80.60      & 81.15      \\ \hline
\textbf{8}                                                                      & 80.25      & \textbf{81.26}      & 79.99      \\ \hline
\textbf{16}                                                                     & 78.70       & 78.38      & 73.82      \\ \bottomrule[1pt]
\end{tabular}
\label{str_trj}
\end{table}

\begin{table}[h]
\centering
\caption{AUC result of MoPRL trained with different pose embedding dimension. Experiment on ShanghaiTech.}
\begin{tabular}{cccc}
\toprule[1pt]
\textbf{Embedding Dimension} & \textbf{64} & \textbf{128} & \textbf{256} \\ \hline
\textbf{AUC on ShanghaiTech} & 76.65       & \textbf{81.26}        & 81.15        \\ \bottomrule[1pt]
\end{tabular}
\label{emb}
\end{table}

%-------------------------------------------------------------------------

%-------------------------------------------------------------------------
\section{Visualization}
In this section, we provide straightforward evidence to demonstrate both the weakness and strength of MoPRL via several visualization illustrations. We further offer a comparison among different methods via visualization to help explain the results in Table 2 in the Paper.

\subsection{ Pose Reconstruction.}
In this section, we compare different reconstruction results between MPED-RNN \cite{park2020learning} and our MoPRL here to elucidate the difference of model capacities. Our ground truth comes from pose estimator \cite{fang2017rmpe}. All poses are extracted from ShanghaiTech dataset. 

\noindent\textbf{Normal Samples.} As mentioned in Section 4.3, we hypothesize that the model capacity of RNN actually limits performance gain from the motion prior. As shown in Figure~\ref{fig:n_pose}, MoPRL can reconstruct normal poses with less reconstruction error, while MPED-RCNN offers poorer ability in recovering normal poses with more significant deviation. We further assume that such deviation shadows the distinction between normality and anomaly brought by the motion prior. 

\noindent\textbf{Abnormal Samples.} As shown in Figure~\ref{fig:ab_pose}, we also provide abnormal cases for intuitive comparison. Compared with the reconstruction on abnormal cases by MPED-RCNN \cite{park2020learning}, the outputs of MoPRL differ the ground truth more in the pose scale rather than shape since we embed motion into pose via scaling. In this case, The abnormal poses are reconstructed with a larger size.

\subsection{Anomaly Score.}

\noindent\textbf{ShanghaiTech.} As shown in Figure~\ref{fig:sht}, in Scene $08\_0157$ and $04\_0050$, both anomalies (skateboarding and balance biking) are related to motion more and correspond to a relatively normal appearance. The performances on both scenes achieve over 98\%. On the contrary, in Scene $08\_0179$, MoPRL fails to capture the skateboarder with a slow speed. And in $01\_0053$, the slow vehicle cheats MoPRL successfully with both occluded pose and regular motion speed. The performances on those two scenes drop to about 60\%, which verifies our discussion in Paper. It demonstrates MoPRL benefits from the proposed Motion Embedder, which strengthens the motion features but still lacks the diversity of motion representation.

\begin{figure}[t]
  \centering
  \includegraphics[width=0.7\linewidth]{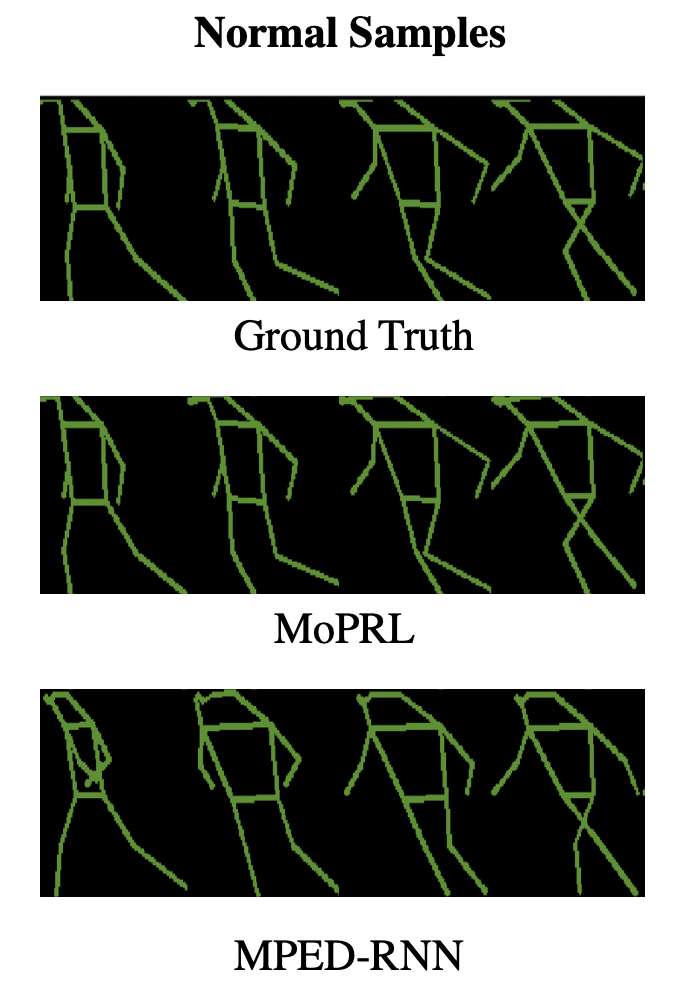}
  \caption{Comparison among ground truth and reconstructed normal pose trajectories from different methods.}
\label{fig:n_pose} 
\end{figure}

\begin{figure}[t]
  \centering
  \includegraphics[width=0.68\linewidth]{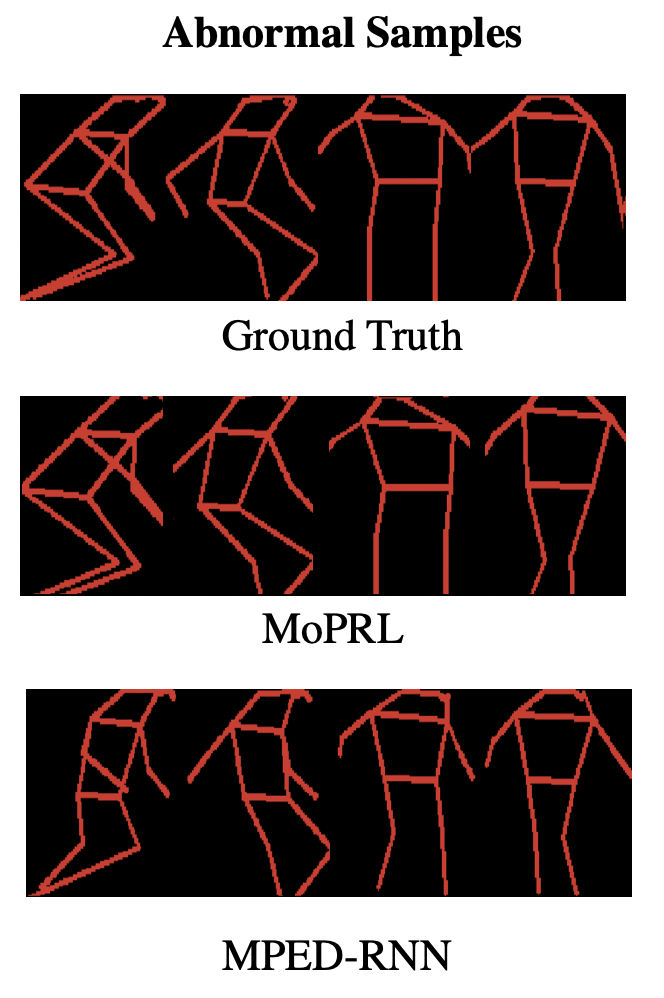}
  \caption{Comparison among ground truth and reconstructed abnormal pose trajectories from different methods.}
\label{fig:ab_pose} 
\end{figure}

\begin{figure*}
  \centering
  \includegraphics[width=0.95\linewidth]{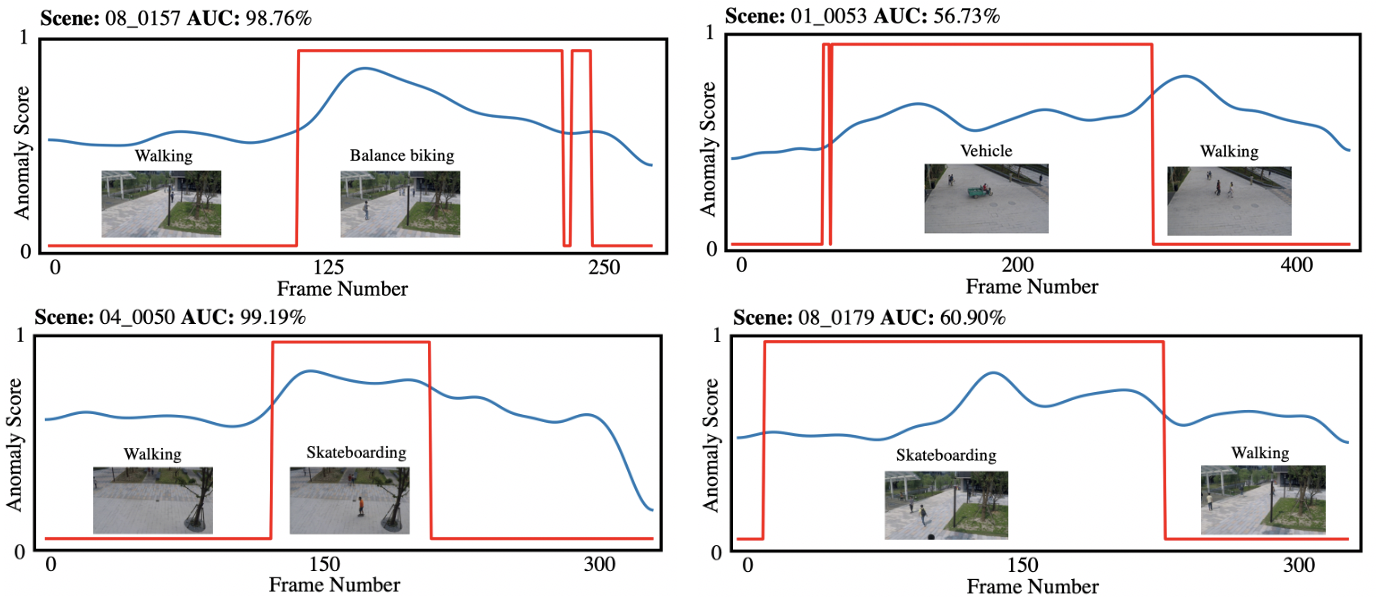}
  \caption{Frame-level anomaly scores (blue lines) corresponding to the labels (red lines) under four scenes in ShanghaiTech dataset. We provide both good (left part) and bad (right part) cases for more discussion. Best viewed in color.}
\label{fig:sht} 
\end{figure*}

\noindent\textbf{Corridor.} As shown in Figure~\ref{fig:corridor}, besides the similar conclusion that MoPRL is sensitive to the motion speed anomaly (like chasing) but fails to capture the motion direction anomaly (like wandering), we observed an interesting difference between Scene $000276$ and $000287$. Both scenes contain the same type of abnormal events that people carry a suspicious object (box) with a normal motion. MoPRL achieves high performance when the object does not occlude the human. When the human is hidden behind the object, the performance decreases sharply. It demonstrates MoRPL can also capture the appearance-related anomaly, and the quality of poses matters a lot to the final performance.

\begin{figure*}
  \centering
  \includegraphics[width=0.95\linewidth]{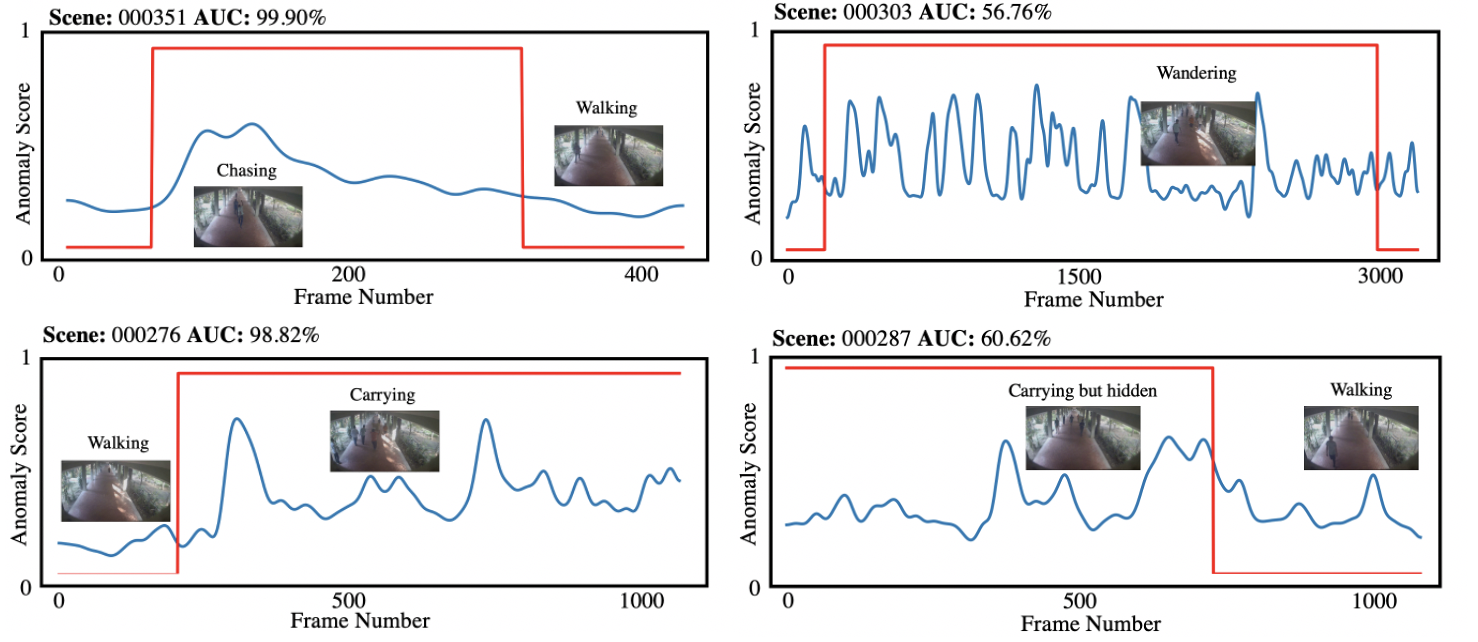}
  \caption{Frame-level anomaly scores (blue lines) corresponding to the labels (red lines) under four scenes in Corridor dataset. We provide both good (left part) and bad (right part) cases for more discussion. Best viewed in color.}
\label{fig:corridor} 
\end{figure*}
